# Supplementary material for: On the Computation of the Zariski Closure of Finitely Generated Groups of Matrices
Source: arXiv:2106.01853 source file (2025-03-03)
Supplement: Supplementary file 1 [file semisimpleappendix.tex]

%\clpistilcommutative*
%
%\begin{proof}
%	Recall that the pistil $P$ is defined to be the intersection of all maximal tori in $\GL_n(\QQbar)$ that contain $\IdComp{G}$.
%    Since $P$ is an intersection of commutative groups, $P$ is itself commutative.
%\end{proof}
%	
%\clpistilbounded*
%
%\begin{proof}
%  Recall that a subgroup of~$\GL_n(\QQbar)$ is a maximal torus if and
%  only if it is conjugate to the group of all diagonal matrices
%  in~$\GL_n(\QQbar)$.  Hence every maximal torus in~$\GL_n(\QQbar)$ is
%  $1$-bounded.  Since $P$ is defined to be the intersection of all
%  maximal tori in~$\GL_n(\QQbar)$ that contain $\IdComp{G}$, it
%  follows that $P$ is $1$-bounded.
%    
%  Since~$G$ is defined over~$\QQ$, it is stable under the action
%  $\Aut(\overline{\QQ}/\QQ)$ on~$\QQ^{n^2+1}$. Now observe that all
%  automorphisms $\sigma\in\Aut(\QQbar/\QQ)$ preserve connectedness,
%  and thus permute the connected components of~$G$. Note also that all
%  automorphisms fix the identity matrix, and therefore must fix the
%  connected component containing it, that
%  is~$\IdComp{G}$. Furthermore, the automorphisms
%  in~$\Aut(\QQbar/\QQ)$ also preserve maximality, and hence permute
%  all maximal tori of~$\QQbar$. It follows that~$P$, being the
%  intersection of all maximal tori of~$\GL_n(\QQ)$, is stable under
%  $\Aut(\QQbar/\QQ)$. Hence,
%  by \cref{lem:bound_k_group_is_k_bounded}\ref{itm:k_bounded}, $P$ is
%  $1$-bounded over~$\QQ$.
%\end{proof}

%\clpistilnormal*
%
%\begin{proof}
%%	Let $N:=\{g\in\GL_n(\overline{\QQ}):gP=Pg\}$ be the normalizer of $P$ in $\GL_n(\QQbar)$; we claim that $G$ normalizes $P$ and hence that $G\leqslant N$.
%%	
%%    To prove the claim, fix $g \in G$.
%
%  Recall that $\IdComp{G}$ is a normal subgroup of~$G$.  Fix $g \in G$
%  and observe that for every maximal torus~$T$ containing
%  $\IdComp{G}$, $gTg^{-1}$ is also a maximal torus, which moreover
%  contains~$\IdComp{G}$ as $g\IdComp{G}g^{-1}=\IdComp{G}$.  We thus
%  see that conjugation by~$g$ induces a bijective self-map on the
%  collection of maximal tori containing~$\IdComp{G}$.  It follows that
%  $gPg^{-1}=P$ for all~$g \in G$, i.e., $G$ normalises~$P$ and hence
%  $G\cap P$ is a normal subgroup of~$G$.
%    
%  To see that $G\cap P$ has finite index in~$G$, recall that
%  $\IdComp{G}$ has finite index in~$G$. Since $\IdComp{G}\subseteq P$,
%  the claim follows.
%\end{proof}

%In order to prove \cref{claim:pistil-quotient-rational}, we need a
%bound on the order of a rational matrix group. It has been
%shown~\cite{KP2002} that a finite subgroup of rational matrices is
%conjugate to a finite subgroup of integer matrices, and furthermore
%the order of any finite subgroup of integer matrices divides
%$(2n)!$~\cite{Newman72,Guralnick2005OrdersOF,BumpusHKST20}. Combining
%these two results yield the bound in~\cref{theo-order-finite-G}.\footnote{%
%Friedland~\cite{Friedland97} showed that the better bound $2^nn!$
%holds for all $n\geqslant72$ but it relies on an incomplete manuscript
%by \cite{Weisfeiler85}.}
%
%\begin{theorem}\label{theo-order-finite-G}
%  For all $n\in \NN$, every finite subgroup of $\GL_{n}(\QQ)$ has
%  order at most $(2n)!$.
%\end{theorem}

%\clqotientrational*
%
%\begin{proof}
%  Let $N:=\{g\in\GL_n(\overline{\QQ}):gP=Pg\}$ be the normaliser
%  of~$P$ in~$\GL_n(\QQbar)$. Since $P$ is defined over~$\QQ$, by
%  quantifier elimination, $N$ is also defined over~$\QQ$.
%	
%  Since $P$ is both $1$-bounded over~$\QQ$
%  (\cref{claim:pistil-bounded}) and a normal subgroup of $N$,
%  by \cref{th:homomorphism_quotient}, there is a homomorphism
%  $\phi_P\colon N\to\GL_p(\QQbar)$, for some $p\leq
%  (n^2+1)^{2}$, such that $\phi_P$ has kernel~$P$ and is defined
%  over~$\QQ$.
%    
%  Recall that in the proof of \cref{claim:pistil-normal-subgroup}, we
%  have shown that $G \leqslant N$, we can thus look at the image
%  of~$G$ under~$\phi_P$. Again
%  following \cref{claim:pistil-normal-subgroup}, since $G\cap P$ has
%  finite index in~$G$, we have that $\phi_P(G)$ is finite.
%    
%  Furthermore, since $G$ is generated over~$\QQ$ and $\phi_P$ is
%  defined over~$\QQ$, the rational points of~$\phi_P(G)$
%  are dense in~$\phi_P(G)$, i.e.,
%  $\Zcl{\phi_P(G)\cap\QQ^{2p+1}}=\phi_P(G)$. Since~$\phi_P(G)$ is finite,
%  $\Zcl{\phi_P(G)\cap\QQ^{2p+1}}=\phi_P(G)\cap\QQ^{2p+1}=\phi_P(G)$ is a finite
%  subgroup of~$\GL_p(\QQ)$.    
%  The claim now follows from \cref{theo-order-finite-G}.
%\end{proof}

%% \clpistilnormalindex*

%% \begin{proof}
%% 	Following \Cref{claim:pistil-quotient-rational}, we have     
%%     \begin{align*}
%%         [G:G\cap P]
%%             &=[PG:P]&&\text{by the second isomorphism theorem\textcolor{red}{ref?}}\\
%%             &=|\phi(G)|\\
%%             &\leq (2(n^2+1)^2)!   &&\qedhere                      
%%     \end{align*}
%%    %which establishes the claim.
%% \end{proof}
