# Supplementary material for: On the Computation of the Zariski Closure of Finitely Generated Groups of Matrices
Source: arXiv:2106.01853 source file (2025-03-03)
Supplement: Supplementary file 2 [file unipotentappendix.tex]

%
%
%
%In order to prove \cref{claim:U-connected-bounded} we recall the
%definition of matrix exponential and matrix
%logarithm~\citep[Sec.~15.1]{HumphreysLAG}. Given a matrix
%$g\in \GL_n(\overline{\QQ})$, its exponential is
%defined by
%\begin{equation*}
%  \exp(g):=\sum_{n=0}^{\infty} \frac{g^n}{n!}\;\:.
%\end{equation*}
%
%A matrix $g'$ is said to be a \emph{matrix logarithm} of~$g$ if $\exp(g) =
% g'$. Since the exponential function is not one-to-one in~$\QQbar$,
% some matrices may have more than one logarithm.  However, for a
% unipotent matrix~$g$ we can define the logarithm uniquely as
%\begin{equation*}
%\log(g)=\sum_{n=1}^{\infty} (-1)^{n-1}\frac{(g-\GId)^n}{n}\;.	
%\end{equation*}
%
%
%\Uconnectedbounded*
%\begin{proof}
%  By~\cite[Lem.~4.3.9]{deGraafBook}, for any $h \in G_u$, there is a
%  unique nilpotent matrix~$\log(h)$ such that $h=\exp(\log(h))$.  We
%  furthermore have that~$\Zcl{\Gen{h}}$ is the image of the map
%  $\Phi_h\colon\overline{\QQ}\rightarrow \GL_n(\overline{\QQ})$ given
%  by $\Phi_h(z) := \exp(z \log(h))$.  Note that~$\Phi_h$ is a
%  polynomial in $z$ of degree at most~$n$ by the nilpotency
%  of~$\log(h)$, hence Zariski-continuous.  It follows
%  that~$\Zcl{\Gen{h}}$ is irreducible.
%    
%  We recall a standard fact that given two irreducible varieties $U$
%        and $V$, the cartesian product $U \times V$ is again
%        irreducible \cite[see, e.g.][Thm.~1.1.9]{deGraafBook}. Since
%        matrix multiplication is a regular map, $\Zcl{U\cdot V}$ is
%        then irreducible as well. Now 
%        from \cref{sub:chains} it follows that any strictly increasing
%  chain of irreducible algebraic subsets of $\GL_n(\overline{\QQ})$
%  has length at most $\dim(\GL_n(\overline{\QQ}))=n^2$.  
%  Thus there
%  exists~$\ell \leq n^2$ and $h_1,\ldots,h_\ell \in G_u$
%  with \[U=\Zcl{\Zcl{\Gen{h_1}}\cdots \Zcl{\Gen{h_\ell}}}=\Zcl{\{ \Phi_{h_1}(z_1) \cdots \Phi_{h_{\ell}}(z_\ell)
%  : z_1,\ldots,z_\ell \in \overline{\QQ} \}} \; .\] In other words, $U$ is the
%  Zariski closure of the image of $\overline{\QQ}^\ell$ under a
%  polynomial map of degree at most~$n^3$ with~$n^2 + 1$ variables
%  defining~$U$ and $\ell$ variables used in the
%  polynomials~$\Phi_{h_i}(z_i)$. Furthermore, by above it follows that $U$ is irreducible.
%  
%%  \textcolor{orange}{As recalled in~\cref{sub:cc},
%%  since~$\overline{\QQ}^\ell$ is irreducible, $U$ is also irreducible.}
%
% 
%  We use \cref{prop:elm=ideal} to eliminate all~$z_i$.  
%  Therefore $U$ is bounded by
%  $(n^3+1)^{2^{(2n^2+1)}} \leq (n^3+1)^{2^{3n^2}}$.  
%  Furthermore, since both $G$ and the collection of unipotent matrices
%  in $\GL_n(\overline{\QQ})$ are stable under
%  $\Aut(\overline{\QQ}/\QQ)$, $U$ is also stable under
%  $\Aut(\overline{\QQ}/\QQ)$.
%  By \cref{lem:bound_k_group_is_k_bounded}\ref{itm:k_bounded}, it
%  follows that $U$ is bounded
%  by $(n^3+1)^{2^{3n^2}}$ over $\QQ$.
%\end{proof}
%
